# Supplementary material for: Fusing Data with Correlations
Source: arXiv:1503.00306 source file (2015-03-01)
Supplement: Supplementary file 1 [file appendix.tex]

\section{Proofs: Section~\ref{sec:fusion_indep}}

\begin{proof}[(Proposition~\ref{prop:sourceQuality})]
    
    We will compare the following correctness probabilities:
        \begin{align*}
            \CPr{\true{t}}{\mO_t}=\frac{1}{1+{1-\alpha \over \alpha}\cdot{1 \over \mu}}\\
            \CPr{\true{t}}{\mO_t'}=\frac{1}{1+{1-\alpha \over \alpha}\cdot{1 \over \mu'}}
        \end{align*}

  We first consider the case that $S'$ is a good source. This means that $r' >
  q'$, where $r'$ is the recall of source $S'$ and $q'$ is its false positive
  rate. 
    
    We consider two cases: that $S'$ provides $t$, and that $S'$ does not
    provide $t$:
    \begin{itemize}
        \item If $\provide{S'}{t}$, then $\mu'=\mu\cdot\frac{r'}{q'}$. Since $r' >
        q'$, from Equation~\eqref{eq:indep} it follows that $\mu'>\mu$, and
        thus, $\CPr{\true{t}}{\mO_t'}>\CPr{\true{t}}{\mO_t}$.
        \item If $\notprovide{S'}{t}$, then $\mu'=\mu\cdot\frac{1-r'}{1-q'}$. Since
        $r' > q'$, it follows that $\mu'<\mu$, and thus,
        $\CPr{\true{t}}{\mO_t'}<\CPr{\true{t}}{\mO_t}$.
    \end{itemize}
    
    If $S'$ is a bad source, then $r'<q'$, and all the above results are inverted.
\end{proof}

\begin{proof}[(Theorem~\ref{thm:pqr})]
    First, the valid range for $q_i$ is $[0,1]$, which means that $\frac{\alpha}{1-\alpha}\cdot\frac{1-p_i}{p_i}\cdot r_i\leq 1$. From this, it directly follows that $\alpha \leq {p_i \over p_i+r_i-p_ir_i}$.
    
    To show the second statement: $p_i > \alpha \Rightarrow \frac{\alpha}{1-\alpha}\cdot\frac{1-p_i}{p_i} < 1 \Rightarrow q_i<r_i$, which means that $S_i$ is a good source.
\end{proof}

\begin{proof}[(Proposition~\ref{prop:tripleProb})]
    
    We will compare the correctness probabilities of a triple $t$, based on
    sources $\mS'$ and $\mS''$:
        \begin{align*}
            \CPr{\true{t}}{\mO_t'}=\frac{1}{1+{1-\alpha \over \alpha}\cdot{1 \over \mu'}}\\
            \CPr{\true{t}}{\mO_t''}=\frac{1}{1+{1-\alpha \over \alpha}\cdot{1 \over \mu''}}
        \end{align*}
        
        We consider the two cases described in the proposition:
        \begin{itemize}
            \item If $\provide{S'}{t}$ and $\provide{S''}{t}$, then
            $\mu'=\mu\cdot\frac{r_{S'}}{q_{S'}}$ and
            $\mu''=\mu\cdot\frac{r_{S''}}{q_{S''}}$. Given $r_{S'}=r_{S''}$ and
            $p_{S'} > p_{S''}$, using Theorem~\ref{thm:pqr} we get $q_{S'} <
            q_{S''}$. Therefore, $\mu'>\mu''$, leading to $\CPr{t}{\mO'_t} >
            \CPr{t}{\mO''_t}$.
            \item If $\notprovide{S'}{t}$ and $\notprovide{S''}{t}$, then
            $\mu'=\mu\cdot\frac{1-r_{S'}}{1-q_{S'}}$ and
            $\mu''=\mu\cdot\frac{1-r_{S''}}{1-q_{S''}}$. Since
            $p_{S'}=p_{S''}>\alpha$,
            $A=\frac{\alpha}{1-\alpha}\cdot\frac{1-p_i}{p_i}<1$. Using
            Theorem~\ref{thm:pqr}, we get:
            \begin{align*}
                \mu'=\mu\cdot\frac{1}{1+(1-A)\frac{r_{S'}}{1-r_{S'}}}\\
                \mu''=\mu\cdot\frac{1}{1+(1-A)\frac{r_{S''}}{1-r_{S''}}}
            \end{align*}
            Since $r_{S'} > r_{S''}$, and $A<1$, it follows that $\mu'<\mu''$
            and hence $\CPr{t}{\mO'_t} < \CPr{t}{\mO''_t}$.\qedhere
        \end{itemize}
\end{proof}

\section{Proofs: Section~\ref{sec:fusion_corr}}

\begin{proof}[(Corollary~\ref{cor:indepEquiv})]
    If all sources are independent, then $r_{1\ldots n}=r_1\cdot
    r_2\cdot\ldots\cdot r_n$, and $r_{12\ldots (i-1)(i+1)\ldots n}=r_1\cdot
    r_2\cdot\ldots r_{(i-1)}\cdot r_{(i+1)}\cdot r_n$. Therefore, all factors
    $C_i^+$ and $C_i^-$ from Equations~\eqref{eq:c_iplus} and
    \eqref{eq:c_iminus} are equal to 1.
\end{proof}

\begin{proof}[(Proposition~\ref{prop:aggrBadCases})]
    If all sources in $\mS$ provide the same data, then the joint recalls of all subsets of sources and the recalls of all individual sources are equal. So, $r_{1\ldots n}=r_{12\ldots(i-1)(i+1)\ldots n}=r_i=r$.  Therefore, $C_i^+=\frac{1}{r}$ for all $i$.  Similarly, $C_i^i=\frac{1}{q}$ for all $i$.  Substituting these values in Equation~\eqref{eq:corr} produces $\mu_{aggr}=1$, leading to $\CPr{t}{\mO_t}=\alpha$.
    
    If all sources are complementary, the joint recall and joint false positive rate for the set of all sources are both zero.  This means that both the numerator and denominator of $\mu_{aggr}$ are 0, leading to a non-valid probability computation. 
    
\end{proof}

\begin{proof}[(Proposition~\ref{prop:runtime})]
    Algorithm~\ref{alg:ptime_corr} iterates over all possible subsets of sources of size $l$ (lines~\ref{ln:term}--\ref{ln:qdiff}).  In the worst case, $\mS_{\bar t}=\mS$, and $l=\lambda$.  So there are ${n \choose \lambda}$ possible subsets.  ${n \choose \lambda}$ is upper bounded by $n^\lambda$.  The process needs to be repeated for all $m$ triples, so the overall computation time of the elastic approximation is $O(m\cdot n^\lambda)$.  There are 2 correlation parameters computed for each iteration of lines~\ref{ln:term}--\ref{ln:qdiff} ($C_{\mS_l}$, $C_{\mS_l}^\neg$), and there are $n$ additional $C_i^+$ and $C_i^-$ parameters.  Overall, the parameters are also bounded by $O(m\cdot n^\lambda)$.
\end{proof}
